# Supplementary material for: Non-standard inference for augmented double autoregressive models with null volatility coefficients
Source: arXiv:1905.01798 ancillary file (2019-05-06)
Supplement: Supplementary file 1 [file Supplementary_material.pdf]

# SUPPLEMENT TO "NON-STANDARD INFERENCE FOR AUGMENTED DOUBLE AUTOREGRESSIVE MODELS WITH NULL VOLATILITY COEFFICIENTS"

Feiyu Jiang*, Dong Li† and Ke Zhu‡

*Tsinghua University*†* and University of Hong Kong*‡

This supplementary material gives the proofs of Theorems 4.2 and 5.1 in Section S1, provides the proofs of Lemmas B.1-B.5 in Section S2, and studies the Bahadur slopes for the Wald, Lagrange multiplier and quasi-likelihood ratio tests in Section S3.

## S1. Proofs of Theorems 4.2 and 5.1.

**Proof of Theorem 4.2.** We only prove (ii), since the proofs of (i) and (iii) are similar to those of Theorem 3.1(i) and (iii). As for (A.5), we have

$$0 = \sqrt{n} I_n(\theta_n) + \sqrt{n} J_n(\theta^*)(\hat{\theta}_{n|3} - \theta_n) + \sqrt{n} K'_\alpha \gamma_{n|3},$$

where $\theta^*$ lies between $\hat{\theta}_{n|3}$ and $\theta_n$. Since $\sqrt{n}(\hat{\theta}_{n|3} - \theta_n) = O_p(1)$ by Theorem 4.1, Lemma B.4(iii) implies that $J_n(\theta^*) = J + o_p(1)$. Then, it follows that

$$o_p(1) = \sqrt{n} I_n(\theta_n) + J\sqrt{n}(\hat{\theta}_{n|3} - \theta_n) + \sqrt{n} K'_\alpha \gamma_{n|3}.$$

Multiplying $K_\alpha J^{-1}$ on both sides of the preceding equality, we can get

$$o_p(1) = \sqrt{n} K_\alpha J^{-1} I_n(\theta_n) + K_\alpha \sqrt{n}(\hat{\theta}_{n|3} - \theta_0 + \theta_0 - \theta_n) + \sqrt{n} K_\alpha J^{-1} K'_\alpha \gamma_{n|3}.$$

Using the facts $K_\alpha(\hat{\theta}_{n|3} - \theta_0) = 0$ and $\sqrt{n}(\theta_n - \theta_0) = h$, it follows that

$$\sqrt{n}\gamma_{n|3} = -\sqrt{n}(K_\alpha J^{-1} K'_\alpha)^{-1} K_\alpha J^{-1} I_n(\theta_n) + (K_\alpha J^{-1} K'_\alpha)^{-1} K_\alpha h + o_p(1).$$

Finally, by Lemma B.4(iii), $J^{-1} I_n(\theta_n) = Z_{n,h} + o_p(1) \to_{\mathcal{L}} Z$, and hence

$$\sqrt{n}\gamma_{n|3} \to_{\mathcal{L}} \mathcal{N}\big((K_\alpha J^{-1} K'_\alpha)^{-1} K_\alpha h,\ (K_\alpha J^{-1} K'_\alpha)^{-1} K_\alpha J^{-1} \Sigma J^{-1} K'_\alpha (K_\alpha J^{-1} K'_\alpha)^{-1}\big),$$

which implies (ii) holds. This completes all of the proofs. □

**Proof of Theorem 5.1.** When model (1.2) is correctly specified, by Theorem 2.1 and the ergodic and dominated convergence theorems, it is not hard to show that

$$\hat{\zeta} \to 0, \qquad \frac{1}{n}\sum_{t=1}^{n}(\hat{\zeta}_t - \bar{\zeta})^2 \to Ew_t^2, \qquad \bar{\xi} \to 0, \qquad \text{and} \qquad \frac{1}{n}\sum_{t=1}^{n}(\hat{\xi}_t - \bar{\xi})^2 \to \bar{\sigma}^2$$

a.s. Hence, it follows that

$$\sqrt{n}(\hat{\rho}_n', \hat{r}_n')' = \sqrt{n}(\tilde{\rho}_n', \tilde{r}_n')' + o_p(1), \tag{S1}$$

where $\tilde{\rho}_n = (\tilde{\rho}_{n1}, \cdots, \tilde{\rho}_{nM})'$ and $\tilde{r}_n = (\tilde{r}_{n1}, \cdots, \tilde{r}_{nM})'$ with $\tilde{\rho}_{nk} = \sum_{t=k+1}^{n} \hat{\zeta}_t\hat{\zeta}_{t-k}/(nEw_t^2)$ and $\tilde{r}_{nk} = \sum_{t=1}^{n} \hat{\xi}_t\hat{\xi}_{t-k}/(n\bar{\sigma}^2)$. Let $\rho_{nk} = \sum_{t=k+1}^{n} \zeta_t\zeta_{t-k}/(nEw_t^2)$ and $r_{nk} = \sum_{t=1}^{n} \xi_t\xi_{t-k}/(n\bar{\sigma}^2)$. Then,

$$\begin{aligned}
\sqrt{n}(\tilde{\rho}_{nk} - \rho_{nk}) &= \frac{1}{\sqrt{n}Ew_t^2}\sum_{t=k+1}^{n} \hat{\zeta}_{t-k}(\hat{\zeta}_t - \zeta_t) + \frac{1}{\sqrt{n}Ew_t^2}\sum_{t=k+1}^{n} \zeta_t(\hat{\zeta}_{t-k} - \zeta_{t-k}) \\
&=: T_{1n}^k + T_{2n}^k, \\
\sqrt{n}(\tilde{r}_{nk} - r_{nk}) &= \frac{1}{\sqrt{n}\bar{\sigma}^2}\sum_{t=k+1}^{n} \hat{\xi}_{t-k}(\hat{\xi}_t - \xi_t) + \frac{1}{\sqrt{n}\bar{\sigma}^2}\sum_{t=k+1}^{n} \xi_t(\hat{\xi}_{t-k} - \xi_{t-k}) \\
&=: T_{3n}^k + T_{4n}^k.
\end{aligned}$$

Since $\|\hat{\theta}_n - \theta_0\| = O_p(1/\sqrt{n})$, by Taylor's expansion, we have

$$\frac{1}{\sqrt{n}}\sum_{t=k+1}^{n} w_{t-k}[\eta_{t-k}(\hat{\theta}_n) - \eta_{t-k}]w_t[\eta_t(\hat{\theta}_n) - \eta_t] = o_p(1),$$

and

$$\frac{1}{\sqrt{n}}\sum_{t=k+1}^{n} w_{t-k}\eta_{t-k}w_t[\eta_t(\hat{\theta}_n) - \eta_t] = -\frac{1}{n}\sum_{t=k+1}^{n} \frac{w_t\mathbf{y}_{t-1}'w_{t-k}\eta_{t-k}}{\sqrt{\alpha_0'\mathbf{x}_{t-1}}}\sqrt{n}(\hat{\phi}_n - \phi_0) + o_p(1),$$

which implies that

$$T_{1n}^k = \frac{1}{Ew_t^2}U_{\rho k}\sqrt{n}(\hat{\theta}_n - \theta_0) + o_p(1).$$

Similarly, we can show that $T_{2n}^k = o_p(1)$, $T_{4n}^k = o_p(1)$ and

$$T_{3n}^k = \frac{1}{\bar{\sigma}^2}U_{rk}\sqrt{n}(\hat{\theta}_n - \theta_0) + o_p(1).$$

Therefore, by (S1) we can obtain that

$$\sqrt{n}(\hat{\rho}_n', \hat{r}_n')' = \sqrt{n}(\rho_n', r_n')' + \left(\frac{1}{Ew_t^2}U_\rho, \frac{1}{\bar{\sigma}^2}U_r\right)'\sqrt{n}(\hat{\theta}_n - \theta_0) + o_p(1). \tag{S2}$$

Next, by the martingale central limit theorem in Brown (1971), we have

$$g_n := \sqrt{n}(\rho_n', r_n', Z_n')' \to_{\mathcal{L}} \mathcal{N}(0, G), \tag{S3}$$

and by the proof of (av) and the fact $J_n = J + o_p(1)$, we have

$$\sqrt{n}(\hat{\theta}_n - \theta_0) = \arg\inf_{\lambda \in \Lambda} \|Z_n - \lambda\|_J + o_p(1). \tag{S4}$$

Then, by (S2)-(S4), $\sqrt{n}(\hat{\rho}_n', \hat{r}_n')' = V\mathcal{G}(g_n) + o_p(1)$. Now, the conclusion holds by the continuous mapping theorem. This completes the proof. □

**S2. Proofs of Lemmas B.1-B.5.**

Let $\mathcal{F}_t$ be the $\sigma$-field generated by $\{y_t, y_{t-1}, \cdots\}$. Recall that $\epsilon_t(\phi) = y_t - \phi \mathbf{y}_{t-1}$. The first and second partial derivatives of $\ell_t(\theta)$ with respect to $\phi$ and $\alpha$ are given as follows:

(i) $\dfrac{\partial \ell_t(\theta)}{\partial \phi} = -\dfrac{\mathbf{y}_{t-1}\epsilon_t(\phi)}{\alpha'\mathbf{x}_{t-1}}$;

(ii) $\dfrac{\partial \ell_t(\theta)}{\partial \alpha} = -\dfrac{\mathbf{x}_{t-1}}{2\alpha'\mathbf{x}_{t-1}}\Big\{\dfrac{\epsilon_t^2(\phi)}{\alpha'\mathbf{x}_{t-1}} - 1\Big\}$;

(iii) $\dfrac{\partial^2 \ell_t(\theta)}{\partial \phi \partial \phi'} = \dfrac{\mathbf{y}_{t-1}\mathbf{y}_{t-1}'}{\alpha'\mathbf{x}_{t-1}}$;

(iv) $\dfrac{\partial^2 \ell_t(\theta)}{\partial \alpha \partial \alpha'} = \dfrac{\mathbf{x}_{t-1}\mathbf{x}_{t-1}'}{2(\alpha'\mathbf{x}_{t-1})^2}\Big\{\dfrac{2\epsilon_t^2(\phi)}{\alpha'\mathbf{x}_{t-1}} - 1\Big\}$;

(v) $\dfrac{\partial^2 \ell_t(\theta)}{\partial \phi \partial \alpha'} = \dfrac{\mathbf{y}_{t-1}\mathbf{x}_{t-1}'\epsilon_t(\phi)}{(\alpha'\mathbf{x}_{t-1})^2}$.

**Proof of Lemma B.1.** We will use facts that $\|\mathbf{x}_{t-1}\| \leq \|\mathbf{z}_{t-1}\|$ and $\|\mathbf{y}_{t-1}\|^2 \leq \sqrt{m+1}\,\|\mathbf{z}_{t-1}\|$ without mentioned.

(i) First, we can show that

$$\begin{aligned} E\sup_{\theta\in\Theta}\Big|w_t \ln(\omega + \sum_{i=1}^q \alpha_i y_{t-i}^2)\Big| \leq & E\sup_{\theta\in\Theta}\Big[I(\omega + \sum_{i=1}^q \alpha_i y_{t-i}^2 \geq 1) w_t \ln(\omega + \sum_{i=1}^q \alpha_i y_{t-i}^2)\Big] \\ & + E\sup_{\theta\in\Theta}\Big[-I(\omega + \sum_{i=1}^q \alpha_i y_{t-i}^2 \leq 1) w_t \ln(\omega + \sum_{i=1}^q \alpha_i y_{t-i}^2)\Big] \\ \leq & E w_t\Big(\bar{\omega} + \bar{\alpha}\sum_{i=1}^q y_{t-i}^2\Big) - E(w_t) I(\underline{\omega} < 1)\ln(\underline{\omega}) < \infty, \end{aligned} \tag{S5}$$

where the last inequality holds by an elementary inequality $\ln x \leq x - 1$ for $x \geq 1$.

Second, since $\epsilon_t(\phi) = y_t - \phi\mathbf{y}_{t-1} = (\phi_0 - \phi)'\mathbf{y}_{t-1} + \eta_t\sqrt{\alpha_0'\mathbf{x}_{t-1}}$, we have $\epsilon_t^2(\phi) \leq 2\eta_t^2(\alpha_0'\mathbf{x}_{t-1}) + 2[(\phi_0 - \phi)'\mathbf{y}_{t-1}]^2$, which entails that

$$\epsilon_t^2(\phi) \leq 2(m+1)^{1/2}\eta_t^2\tilde{\alpha}\,\|\mathbf{x}_{t-1}\| + 8(m+1)^{3/2}\bar{\phi}^2\,\|\mathbf{z}_{t-1}\|, \tag{S6}$$

where $\tilde{\alpha} = \max(\bar{\alpha}, 1)$. Since $\eta_t \in \mathcal{F}_t$ is independent of $\{w_t, \mathbf{x}_{t-1}, \mathbf{y}_{t-1}\}$ and $\omega \geq \underline{\omega} > 0$, it follows that

$$E \sup_{\theta \in \Theta} \frac{w_t \epsilon_t^2(\phi)}{\omega + \sum_{i=1}^q \alpha_i y_{t-i}^2} \leq CE\{w_t \|\mathbf{z}_{t-1}\|\} < \infty. \tag{S7}$$

By (S5) and (S7), we know that (i) holds.

(ii) & (iii) By (S6), Assumption 2.2 and a similar argument as for (i), we can show that

$$\begin{aligned}
E \sup_{\theta \in \Theta} \left\| w_t \frac{\partial \ell_t(\theta)}{\partial \phi} \right\| &\leq CE \sup_{\theta \in \Theta} \left\| w_t \mathbf{y}_{t-1}(1 + |\eta_t|) \|\mathbf{z}_{t-1}\|^{1/2} \right\| \leq CE(w_t \|\mathbf{z}_{t-1}\|) < \infty, \\
E \sup_{\theta \in \Theta} \left\| w_t \frac{\partial \ell_t(\theta)}{\partial \alpha} \right\| &\leq CEw_t(\|\mathbf{z}_{t-1}\| + \|\mathbf{z}_{t-1}\|^2) < \infty, \\
E \sup_{\theta \in \Theta} \left\| w_t \frac{\partial^2 \ell_t(\theta)}{\partial \phi \partial \phi'} \right\| &\leq CE\{w_t \|\mathbf{z}_{t-1}\|\} < \infty, \\
E \sup_{\theta \in \Theta} \left\| w_t \frac{\partial^2 \ell_t(\theta)}{\partial \alpha \partial \alpha'} \right\| &\leq CE\Big\{ \sup_{\theta \in \Theta} \|w_t \mathbf{x}_{t-1} \mathbf{x}_{t-1}'\| \Big\} + CE\Big\{ \sup_{\theta \in \Theta} w_t \epsilon_t(\phi)^2 \|\mathbf{x}_{t-1} \mathbf{x}_{t-1}'\| \Big\} \\
&\leq CEw_t(\|\mathbf{z}_{t-1}\|^2 + \|\mathbf{z}_{t-1}\|^3) < \infty, \\
E \sup_{\theta \in \Theta} \left\| w_t \frac{\partial^2 \ell_t(\theta)}{\partial \phi \partial \alpha'} \right\| &\leq CE\{w_t \|\mathbf{z}_{t-1}\|^2\} < \infty.
\end{aligned}$$

Thus, it follows that (ii) and (iii) hold. □

**Proof of Lemma B.2.** (i) First, we show that if there exist two vectors $a \in \mathbb{R}^p, b \in \mathbb{R}^{q+1}$ such that $a'\mathbf{y}_{t-1} = b'\mathbf{x}_{t-1} = 0$ a.s., then $a = 0$ and $b = 0$. Otherwise, suppose $a \neq 0$, e.g., say that $a_1 = 1$. Then, $y_t = -\sum_{i=2}^p a_i y_{t-i+1}$ a.s., and hence $E\eta_t^2 = E(\eta_t(-\sum_{i=2}^p a_i y_{t-i+1} - \phi_0'\mathbf{y}_{t-1})/\sqrt{\alpha_0'\mathbf{x}_{t-1}}) = 0$ since $\eta_t$ is independent of $\mathcal{F}_{t-1}$. This is a contradiction. Thus, $a = 0$. Similarly, $b = 0$.

Second, by Lemma B.1(i),

$$\begin{aligned}
E[w_t \ell_t(\theta)] =& \frac{1}{2} E\Big[ w_t \ln(\alpha'\mathbf{x}_{t-1}) + w_t \frac{(y_t - \phi'\mathbf{y}_{t-1})^2}{\alpha'\mathbf{x}_{t-1}} \Big] \\
=& \frac{1}{2} \Big[ Ew_t \ln(\alpha'\mathbf{x}_{t-1}) + E\Big( w_t \frac{\alpha_0'\mathbf{x}_{t-1}}{\alpha'\mathbf{x}_{t-1}} \Big) \Big] + \frac{1}{2} E\Big[ w_t \frac{((\phi - \phi_0)'\mathbf{y}_{t-1})^2}{\alpha'\mathbf{x}_{t-1}} \Big].
\end{aligned} \tag{S8}$$

The first term in (S8), omitting the scale factor 1/2, can be rearranged as

$$E\Big[ w_t \ln(\alpha'\mathbf{x}_{t-1}) + w_t \frac{\alpha_0'\mathbf{x}_{t-1}}{\alpha'\mathbf{x}_{t-1}} \Big] = [Ew_t(M_t - \ln M_t)] + E\{w_t \ln(\alpha_0'\mathbf{x}_{t-1})\},$$

where $M_t = \alpha_0'\mathbf{x}_{t-1}/(\alpha'\mathbf{x}_{t-1})$. Note that the function $g(x) = x - \ln x \geq 0$ for $x > 0$ has a minimum at $x = 1$. When $M_t = 1$ a.s., then $E[w_t g(M_t)] = Ew_t$. If $\mathbb{P}(M_t = 1) \neq 1$, then $\mathbb{P}(g(M_t) > g(1)) \neq 0$ so that $E[w_t g(M_t)] > E[w_t g(1)] = Ew_t$. Thus, in order for the first

term to obtain the minimum, $M_t = 1$ a.s., which in turn implies that $\alpha = \alpha_0$. Clearly, the second term in (S8) is minimized at $\phi = \phi_0$. Therefore, $E[w_t \ell_t(\theta)]$ is minimized at $\theta = \theta_0$.

(ii) By Lemma B.1(ii) and Taylor's expansion, it is straightforward to see that (ii) holds. This completes all of the proofs. □

**Proof of Lemma B.3.** See Example 4 in Section 3 of Andrews (1988). □

**Proof of Lemma B.4.** (i) It follows by the same arguments as for Lemma B.2(i).

(ii) By Lemma B.1(iii), it follows easily that for any $\theta \in \Theta$, $\|E[J_n(\theta)]\| < \infty$. Then, by Assumption 2.1 and the uniform law of large numbers, we have

$$\sup_{\theta\in\Theta} \|J_n(\theta) - E[J_n(\theta)]\| = o_p(1). \tag{S9}$$

Since $EJ_n(\theta)$ is continuous, we have $EJ_n(\theta_n^*) \to EJ_n(\theta_0) = J$, which together with (S9), we can show that $\|J_n(\theta_n^*) - J\| = o_p(1)$. Similarly, we can prove that $\|\Sigma_n(\theta_n^*) - \Sigma\| = o_p(1)$ and $\|D_n(\theta_n^*) - D\| = o_p(1)$. Clearly, $Z_n \to_{\mathcal{L}} Z$ follows by the martingale central limit theorem in Brown (1971).

(iii) Under $\mathbb{P}_{n,h}$, we write

$$J_n(\theta_n^*) = \frac{1}{n}\sum_{t=1}^n w_{t,n}\frac{\partial^2 l_{t,n}(\theta_n^*)}{\partial\theta\partial\theta'} = \frac{1}{n}\sum_{t=1}^n \begin{pmatrix} J_{n,h,t}^{(1,1)}(\theta_n^*) & J_{n,h,t}^{(1,2)}(\theta_n^*) \\ J_{n,h,t}^{(1,2)'}(\theta_n^*) & J_{n,h,t}^{(2,2)}(\theta_n^*) \end{pmatrix},$$

where

$$J_{n,h,t}^{(1,1)}(\theta) = w_{t,n}\frac{\partial^2 \ell_{t,n}(\theta)}{\partial\phi\partial\phi'},\quad J_{n,h,t}^{(1,2)}(\theta) = w_{t,n}\frac{\partial^2 \ell_{t,n}(\theta)}{\partial\phi\partial\alpha'},\quad \text{and}\quad J_{n,h,t}^{(2,2)}(\theta) = w_{t,n}\frac{\partial^2 \ell_{t,n}(\theta)}{\partial\alpha\partial\alpha'}.$$

By Assumption 2.3$'$ with $\delta = 2$ and the similar arguments as for Lemma B.1, we can show that

$$\begin{aligned}
\left\|J_{n,h,t}^{(1,1)}(\theta)\right\| &= \left\|w_{t,n}\frac{\mathbf{y}_{t-1,n}\mathbf{y}_{t-1,n}'}{\alpha'\mathbf{x}_{t-1,n}}\right\| \le Cw_{t,n}\|\mathbf{z}_{t-1,n}\| < \infty,\\
\left\|J_{n,h,t}^{(1,2)}(\theta)\right\| &= \left\|w_{t,n}\frac{\mathbf{y}_{t-1,n}\mathbf{x}_{t-1,n}\epsilon_{t,n}(\theta)}{(\alpha'\mathbf{x}_{t-1,n})^2}\right\| \le C\{w_{t,n}\|\mathbf{z}_{t-1,n}\|^3(1+\eta_t^2)\} < \infty,\\
\left\|J_{n,h,t}^{(2,2)}(\theta)\right\| &= \left\|w_{t,n}\frac{\mathbf{x}_{t-1,n}\mathbf{x}_{t-1,n}'}{2(\alpha'\mathbf{x}_{t-1,n})^2}\frac{\alpha'\mathbf{x}_{t-1,n} - 2\epsilon_{t,n}^2(\theta)}{\alpha'\mathbf{x}_{t-1,n}}\right\|\\
&\le C(\left\|w_{t,n}\mathbf{x}_{t-1,n}\mathbf{x}_{t-1,n}'\right\| + \left\|w_{t,n}\epsilon_{t,n}(\theta)^2\mathbf{x}_{t-1,n}\mathbf{x}_{t-1,n}'\right\|)\\
&\le C\{w_{t,n}\|\mathbf{z}_{t-1,n}\|^2 + \|\mathbf{z}_{t-1,n}\|^3(1+\eta_t^2)\} < \infty,
\end{aligned}$$

which imply that all of $J_{n,h,t}^{(1,1)}(\theta)$, $J_{n,h,t}^{(1,2)}(\theta)$ and $J_{n,h,t}^{(2,2)}(\theta)$ are $L^s$ uniformly bounded with $s = 3/2$.

Moreover, for any $\theta$, $\tilde{\theta}$, and $1 \le i, j, k \le p+q+2$, Taylor's expansion implies that

$$\frac{\partial^2 F_n(\theta)}{\partial\theta_i \partial\theta_j} - \frac{\partial^2 F_n(\tilde{\theta})}{\partial\tilde{\theta}_i \partial\tilde{\theta}_j} = (\theta - \tilde{\theta})' \frac{\partial^3 F_n(\theta^*)}{\partial\theta \partial\theta_i \partial\theta_j},$$

where $\theta^*$ lies between $\theta$ and $\tilde{\theta}$. By Assumption 2.3$'$ with $\delta = 2$, it is not hard to see that

$$E \sup_{\theta \in \Theta} \left\| \frac{\partial^3 F_n(\theta)}{\partial\theta_k \partial\theta_i \partial\theta_j} \right\| < \infty.$$

Hence, by the similar arguments as for (A.11), we can show that $\sup_{\theta\in\Theta} \|J_n(\theta) - J\| = o_p(1)$, which implies that $\|J_n(\theta_n^*) - J\| = o_p(1)$. Similarly, we can prove that $\|\Sigma_n(\theta_n^*) - \Sigma\| = o_p(1)$ and $\|D_n(\theta_n^*) - D\| = o_p(1)$. By the Cramér-Wold device and the martingale central limit theorem in Brown (1971), $\sqrt{n} I_n(\theta_n) \to_{\mathcal{L}} \Sigma$, which follows that $Z_{n,h} \to_{\mathcal{L}} Z$. This completes all of the proofs. □

**Proof of Lemma B.5.** The proof is similar to the one of Lemma B.4 in Pedersen (2017). □

**S3. Bahadur slope.** In this section, we measure the efficiency of all three tests by considering the Bahadur slopes under the fixed alternative:

$$H_1 : \theta_0^{(3)} > 0.$$

Let $S_W(x) = \mathbb{P}(W > x)$, $S_L(x) = \mathbb{P}(L > x)$ and $S_Q(x) = \mathbb{P}(Q > x)$ be the asymptotic survival functions of the Wald, LM and QLR statistics under $H_0$, respectively. Moreover, suppose that

$$\theta_{0|3} = \arg \inf_{\theta\in\Theta:\theta_0^{(3)} = \mathbf{0}^{d_3}} E(w_t \ell_t(\theta)) \tag{S10}$$

exists and is unique, and let

$$M_{0|3} = E\left(w_t \frac{\partial \ell_t(\theta_{0|3})}{\partial\theta}\right), \quad J_{0|3} = E\left(w_t \frac{\partial^2 \ell_t(\theta_{0|3})}{\partial\theta\partial\theta'}\right), \quad \Sigma_{0|3} = E\big(w_t \Gamma_t(\theta_{0|3})' D_{0|3} \Gamma_t(\theta_{0|3})\big),$$

where $D_{0|3} = \lim_{n\to\infty} \hat{D}_{n|3}$.

Theorem S1. *Suppose that Assumptions 2.1-2.4 and (S10) hold. Then, under $H_1$,*

(i) *the approximate Bahadur slope of the Wald test is:*

$$\lim_{n\to\infty} -\frac{2}{n} \log S_W(W_n) = \theta_0^{(3)'} (K_\alpha J^{-1} \Sigma J^{-1} K'_\alpha) \theta_0^{(3)};$$

(ii) *the approximate Bahadur slope of the LM test is:*

$$\lim_{n\to\infty} -\frac{2}{n}\log S_L(L_n) = M_{0|3}' J_{0|3}^{-1} K_\alpha' \{K_\alpha J_{0|3}^{-1}\Sigma_{0|3} J_{0|3}^{-1} K_\alpha'\}^{-1} K_\alpha J_{0|3}^{-1} M_{0|3};$$

(iii) *when $d_2 = 0$, the approximate Bahadur slope of the QLR statistic is*

$$\lim_{n\to\infty} -\frac{2}{n}\log S_Q(Q_n) = \frac{2}{c} E\{w_t[\ell_t(\theta_{0|3}) - \ell_t(\theta_0)]\}$$

*for some constant $c \in [D_{\min}, D_{\max}]$, where $D_{\min}$ and $D_{\max}$ are two eigenvalues of $D$.*

*In addition, these three tests are consistent.*

Remark S1. *When $d_2 = 0$, the proof of Theorem S1 below shows that*

$$Q = cW \tag{S11}$$

*for some constant $c \in [D_{\min}, D_{\max}]$. As a special case that $\kappa_3 = 0$ and $\kappa_4 = 3$ (e.g., $\eta_t \sim \mathcal{N}(0,1)$), we have $c = 1$, and this coincides with Proposition 2 in Francq and Zakoïan (2009). In general, the result in (S11) is different from Proposition 2 in Francq and Zakoïan (2009) due to the presence of conditional mean coefficients.*

*When $d_2 \neq 0$, the result in (S11) will not hold due to the term $\lambda_{|3}^{\Lambda'}\Xi\lambda_{|3}^{\Lambda'}$, making it hard to cope with the approximate Bahadur slope of the QLR statistic.*

The Bahadur slope measures the rate of convergence of $p$-value, and usually a test is considered more efficient than another one when its slope is greater. As in Francq and Zakoïan (2009), a formal comparison of Bahadur slopes for all considered tests is not easy, since $J$, $J_{0|3}$, $\Sigma$ and $\Sigma_{0|3}$ are unknown in closed form, particularly when the self-weighted function $w_t$ is included.

**Proof of Theorem S1.** By (S10) and Theorem 3.1 in White (1982), we can show that $\hat{\theta}_{n|3} \to \theta_{0|3}$ as $n \to \infty$.

(i) Under $H_1$, we have

$$\lim_{n\to\infty} W_n/n = \theta_0^{(3)'}\{K_\alpha J^{-1}\Sigma J^{-1} K_\alpha'\}^{-1}\theta_0^{(3)}. \tag{S12}$$

Let $K_i$'s be the matrices constructed by canceling several (up to $d_2 + d_3 - 1$) rows of $K$, and $P_i = I_d - J^{-1}K_i'(K_i J^{-1} K_i')^{-1} K_i$. Then, by the same argument as for (5) in Francq and Zakoïan (2007), we can deduce that

$$\|\lambda^\Lambda\|_\Omega^2 = \|Z\|_\Omega^2 1_\Lambda(Z) + \sum_{i=1}^{2^{(d_2+d_3)}-1} \|P_i Z\|_\Omega^2 1_{\mathcal{D}_i}(Z), \tag{S13}$$

which entails that

$$S_W(x) = \mathbb{P}(\|\lambda^\Lambda\|_\Omega^2 > x) = \mathbb{P}\Big(\|Z\|_\Omega^2 1_\Lambda(Z) + \sum_{i=1}^{2^{(d_2+d_3)}-1} \|P_i Z\|_\Omega^2 1_{\mathcal{D}_i}(Z) > x\Big),$$

where $\Lambda = \{\lambda \in \mathbb{R}^d | K\lambda \geq 0\}$ and $\{\mathcal{D}_i\}$ forms a partition of $\mathbb{R}^d - \Lambda$.

On one hand, since $\|P_i Z\|_\Omega^2 \leq \|Z\|_\Omega^2$, it follows that

$$\log S_W(x) \leq \log \mathbb{P}(\|Z\|_\Omega^2 > x) = \log \mathbb{P}\big(\|Z_{(3)}\|^2_{[\mathrm{var}(Z_{(3)})]^{-1}} > x\big) = \log \mathbb{P}(\chi^2_{d_3} > x). \tag{S14}$$

On the other hand,

$$\begin{aligned}
\log S_W(x) &\geq \log \mathbb{P}(\|Z\|_\Omega^2 1_\Lambda(Z) > x) \\
&= \log \mathbb{P}(\|Z_3\|^2_{[\mathrm{var}(Z_3)]^{-1}} 1_{Z_{(2,3)}\geq 0} > x) \\
&= \log \mathbb{P}(\|Z_3\|^2_{[\mathrm{var}(Z_3)]^{-1}} > x | Z_{(2,3)} \geq 0) + \log \mathbb{P}(Z_{(2,3)} \geq 0) \\
&= \log \mathbb{P}(\|Z_3\|^2_{[\mathrm{var}(Z_3)]^{-1}} > x) + \log \mathbb{P}(Z_{(2,3)} \geq 0) \\
&= \log \mathbb{P}(\chi^2_{d_3} > x) + \log \mathbb{P}(Z_{(2,3)} \geq 0),
\end{aligned} \tag{S15}$$

where the second equality holds by the symmetric law of $Z$. Thus, by (S12), (S14)-(S15) and the fact that $\log \mathbb{P}(\chi^2_{d_3} > x) \sim -x/2$ as $x \to \infty$, we can show that (i) holds.

(ii) By the law of large numbers and the continuous mapping theorem, it follows that

$$\frac{L_n}{n} = M'_{0|3} J^{-1}_{0|3} K'_\alpha \{K_\alpha J^{-1}_{0|3} \Sigma_{0|3} J^{-1}_{0|3} K'_\alpha\}^{-1} K_\alpha J^{-1}_{0|3} M_{0|3} + o_p(1).$$

Then, (ii) holds by the fact that $L \sim \chi^2_{d_3}$ and $\log \mathbb{P}(\chi^2_{d_3} > x) \sim -x/2$ as $x \to \infty$.

(iii) Since $\hat{\theta}_{n|3} \to \theta_{0|3}$ and $\hat{\theta}_n \to \theta_0$ (a.s.), by Taylor's expansion and Lemma B.4(ii), we can show that

$$\begin{aligned}
F_n(\hat{\theta}_{n|3}) =& F_n(\theta_{0|3}) + I_n(\theta_{0|3})'(\hat{\theta}_{n|3} - \theta_{0|3}) + \frac{1}{2}(\hat{\theta}_{n|3} - \theta_{0|3})' J_{0|3}(\hat{\theta}_{n|3} - \theta_{0|3}) + o_p(1), \\
F_n(\hat{\theta}_n) =& F_n(\theta_0) + I_n(\theta_0)'(\hat{\theta}_n - \theta_0) + \frac{1}{2}(\hat{\theta}_n - \theta_0)' J(\hat{\theta}_n - \theta_0) + o_p(1).
\end{aligned}$$

Hence, since $I_n(\theta_{0|3}) = O_p(1)$ and $I_n(\theta_0) = O_p(1)$, it follows that

$$\frac{Q_n}{n} = 2\{F_n(\theta_{0|3}) - F_n(\theta_0)\} + o_p(1) = 2E\{w_t[\ell_t(\theta_{0|3}) - \ell_t(\theta_0)]\} + o_p(1). \tag{S16}$$

When $d_2 = 0$, we have $K_\alpha = K$, $\Omega = K'(KJ^{-1}\Sigma J^{-1}K')^{-1}K$ and

$$Q = \|\lambda^\Lambda\|_\Xi^2 = \|Z\|_\Xi^2\, 1_\Lambda(Z) + \sum_{i=1}^{2^{d_3}-1} \|P_i Z\|_\Xi^2 1_{\mathcal{D}_i}(Z), \tag{S17}$$

where (S17) holds by a similar argument as for (S13). Denote the largest and smallest eigenvalues of $D$ by $D_{\max}$ and $D_{\min}$, respectively. Then, $D_{\min}J \leq \Sigma \leq D_{\max}J$, where $B \leq A$ means $(A - B)$ is semi-positive definite. Thus, it follows that

$$\text{(S18)} \qquad \frac{1}{D_{\max}}\Xi \leq \Omega \leq \frac{1}{D_{\min}}\Xi.$$

Next, by (S13) and (S17), we have

$$\begin{aligned} D_{\max}W - Q &= D_{\max}\left\|\lambda^{\Lambda}\right\|_{\Omega}^{2} - \left\|\lambda^{\Lambda}\right\|_{\Xi}^{2} \\ &= \|Z\|_{D_{\max}\Omega}^{2} 1_{\Lambda}(Z) + \sum_{i=1}^{2^{d_3}-1} \|Z\|_{P_i' D_{\max}\Omega P_i}^{2} 1_{\mathcal{D}_i}(Z) - \|Z\|_{\Xi}^{2} 1_{\Lambda}(Z) - \sum_{i=1}^{2^{d_3}-1} \|Z\|_{P_i'\Xi P_i}^{2} 1_{\mathcal{D}_i}(Z) \\ &= \|Z\|_{D_{\max}\Omega-\Xi}^{2} 1_{\Lambda}(Z) + \sum_{i=1}^{2^{d_3}-1} \|Z\|_{P_i'(D_{\max}\Omega-\Xi)P_i}^{2} 1_{\mathcal{D}_i}(Z) \geq 0, \end{aligned}$$

where the inequality holds since $D_{\max}\Omega - \Xi > 0$ by (S18). Similarly, we can show that $Q - D_{\min}W \geq 0$. Hence, we can conclude that $Q = cW$ for some constant $c \in [D_{\min}, D_{\max}]$, and then by part (i) we have

$$\text{(S19)} \qquad \log \mathbb{P}(Q > x) = \log \mathbb{P}(W > x/c) \sim -x/2c \text{ as } x \to \infty.$$

Now, by (S16) and (S19), we know that (iii) holds. This completes all of the proofs. □

**References.**


Andrews, D.W.K., 1988. Laws of large numbers for dependent non-identically distributed random variables. Econometric Theory 4, 458–467.

Brown, B.M., 1971. Martingale central limit theorems. Ann. Math. Statist. 42, 59–66.

Francq, C., Zakoïan, J.-M., 2007. Quasi-maximum likelihood estimation in GARCH processes when some coefficients are equal to zero. Stochastic Process. Appl. 117, 1265–1284.

Francq, C., Zakoïan, J.-M., 2009. Testing the nullity of GARCH coeffcients: correction of the standard tests and relative effciency comparisons. J. Amer. Statist. Assoc. 104, 313–324.

Pedersen, R.S., 2017. Inference and testing on the boundary in extended constant conditional correlation GARCH models. J. Econometrics 196, 23–36.

White, H., 1982. Maximum likelihood estimation of misspecified models. Econometrica 50, 1–25.



Center for Statistical Science
and Department of Industry Engineering
Tsinghua University
Beijing 100084, China
E-mail: jfy16@mails.tsinghua.edu.cn
malidong@tsinghua.edu.cn

Department of Statistics & Actuarial Science
The University of Hong Kong
Hong Kong
E-mail: mazhuke@hku.hk
